# Supplementary material for: Camera Alignment and Weighted Contrastive Learning for Domain Adaptation in Video Person ReID
Source: arXiv:2211.03626 source file (2022-11-07)
Supplement: Supplementary file 1 [file SuppMaterial.tex]

\subsection{Visualizations}

    In this section, activation map visualizations are represented. Figure \ref{fig:actmap} represents the better localization for the features across the proposed method. Compared to the baseline SPCL, less background information is captured and allow the model to focus properly on strong identity-based features.

    \begin{figure*}[!ht]
         \centering
         \includegraphics[width=0.9\textwidth]{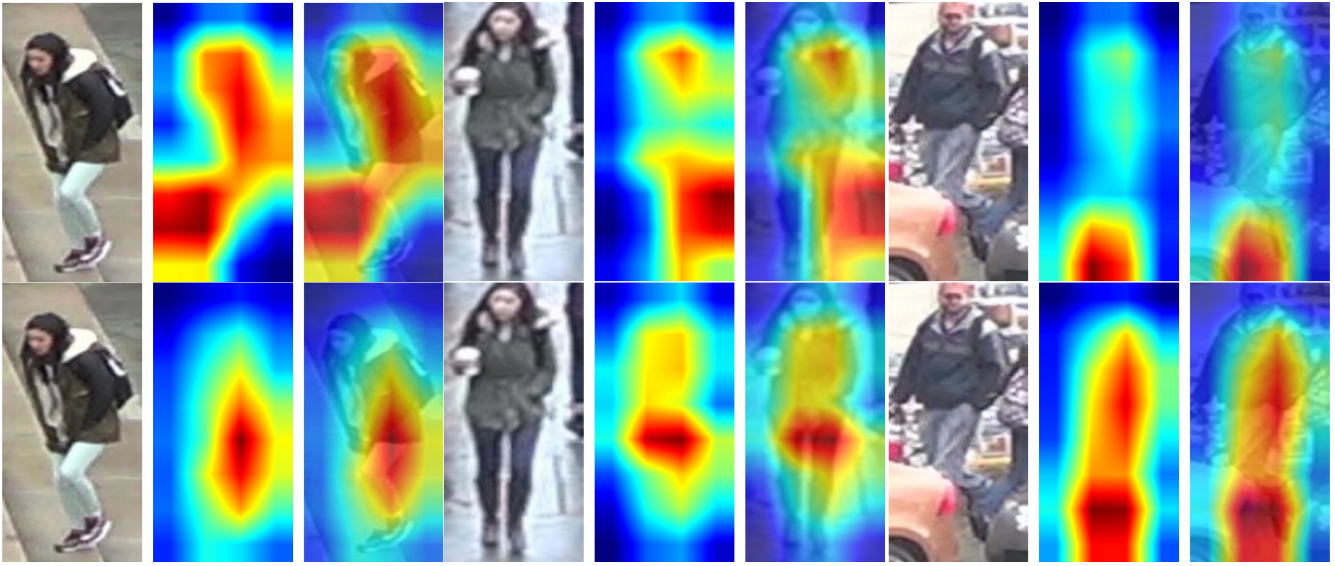}
         \caption{Three individuals from the target represented. Top is from the baseline SPCL and bottom is our proposed approach. The first image represent the sample, the middle is the activation map and the last image is the superposition of the sample with the activation map.}
        \label{fig:actmap}
    \end{figure*}
     
\subsection{Impact of the number of frames per Tracklets}

    This section deals with the number of frames per tracklet. We can observe Table \ref{tab:frames_per_tracklet} that since we cut each tracklet in equal chunks to maintain scalability to all the dataset, the temporal information remains stable from 4 frames per tracklets and so performances does not differ much. In this context, we assume that keeping the number of frames per tracklets to the minimal acceptable value (4 in our case) is suitable for high memory consumption task (i.e. video-based ReID).
    
    \begin{table}[!ht]
        \begin{tabular}{|c|cc|cc|cc|}
            \hline
            \multirow{Number of frames per tracklet} & \multicolumn{2}{c|}{PRID2011}      & \multicolumn{2}{c|}{iLIDS-VID}     & \multicolumn{2}{c|}{MARS}          \\ \cline{2-7} 
                                                           & \multicolumn{1}{c|}{mAP}  & Rank-1 & \multicolumn{1}{c|}{mAP}  & Rank-1 & \multicolumn{1}{c|}{mAP}  & Rank-1 \\ \hline
            2                                              & \multicolumn{1}{c|}{89.2} & 91.6   & \multicolumn{1}{c|}{74.5} & 80.4   & \multicolumn{1}{c|}{83.8} & 77.0   \\ \hline
            4                                              & \multicolumn{1}{c|}{92.1} & 94.5   & \multicolumn{1}{c|}{76.0} & 84.0   & \multicolumn{1}{c|}{86.9} & 81.8   \\ \hline
            8                                              & \multicolumn{1}{c|}{91.9} & 94.2   & \multicolumn{1}{c|}{76.2} & 84.0   & \multicolumn{1}{c|}{86.6} & 80.6   \\ \hline
            16                                             & \multicolumn{1}{c|}{92.0} & 94.9   & \multicolumn{1}{c|}{75.7} & 84.2   & \multicolumn{1}{c|}{87.1} & 81.3   \\ \hline
        \end{tabular}
        \label{tab:frames_per_tracklet}
        \caption{Results for a supervised training using different frames per tracklets. }
    \end{table}
